# Supplementary material for: Ultrafast Optical Control of Magnetic Order and Fermi Surface Topology at a Quantum Critical Point
Source: arXiv:2106.08220 ancillary file (2021-06-15)
Supplement: Supplementary file 1 [file supp.pdf]

# Supplemental Material for *Ultrafast Optical Control of Magnetic Order and Fermi Surface Topology at a Quantum Critical Point*

Benedikt Fauseweh,[1] Jian-Xin Zhu[1,2]

[1] *Theoretical Division, Los Alamos National Laboratory, Los Alamos, New Mexico 87545, USA*

[2] *Center for Integrated Nanotechnologies, Los Alamos National Laboratory, Los Alamos, New Mexico 87545, USA*

## Time-dependent Variational Monte Carlo Results

In order to verify our results with an independent method, we use time-dependent variational Monte Carlo (td-VMC) to simulate the effect of strong laser pulses within the paramagnetic regime of the square lattice Kondo model. We investigate an $8$ by $8$ lattice with periodic-anti-periodic boundary conditions to fulfill the closed shell condition. The VMC ground state phase diagram is qualitatively similar to the mean-field phase diagram, but the quantum phase transition is at lower $J$ due to the exact suppression of charge degrees of freedom on the $f$ lattice sites. It was shown in [1], that the PM/AFM phase transition is at $J \approx 1.35 t_{\text{hop}}$ for $n_c \approx 0.9$. Since we are working with a electron conserving wave function, we use $60$ electrons, corresponding to $n_c = 0.9375$ and start from the ground state wave function at $J = 1.6 t_{\text{hop}}$. For the details on the variational wave function used we refer to the main text. To quantify the tendency to form magnetic order we compute the spin structure factor

$$S_S(\mathbf{k}) = \frac{1}{N_{\text{S}}} \sum_{i,j} \langle \mathbf{S}_i \cdot \mathbf{S}_j \rangle \, e^{i\mathbf{q}(\mathbf{r}_i - \mathbf{r}_j)}. \tag{1}$$

The result for the spin structure factor in equilibrium is shown in Fig. 1. The strong peak at $\mathbf{k_c} = (\pi, \pi)$ is indicative for strong antiferromagnetic correlations. However, at this strong Kondo coupling it was shown in [1], that the correlation is not yet sufficient to form long range order. As in the main text, we perturb the ground state with a short laser pulse $A(t) = A_0 \exp(-(t - t_c)^2/2t_d^2) \cos(\omega_0(t - t_c))$, where $t_c = 15/t_{\text{hop}}$ is the pulse center, $t_d = 5/t_{\text{hop}}$ is the pulse width, $A_0 = 0.15$ is the overall pulse amplitude and $\omega_0 = 0.1$. We then track the peak height of the spin structure factor as function of time $t$ in Fig. 2. The peak is strongly affected by the laser pulse and increases on average after the pulse, thus enhancing the tendency to form magnetic order. Due to the heavy numerical cost of each tVMC run, it is not possible to obtain a similar dynamical

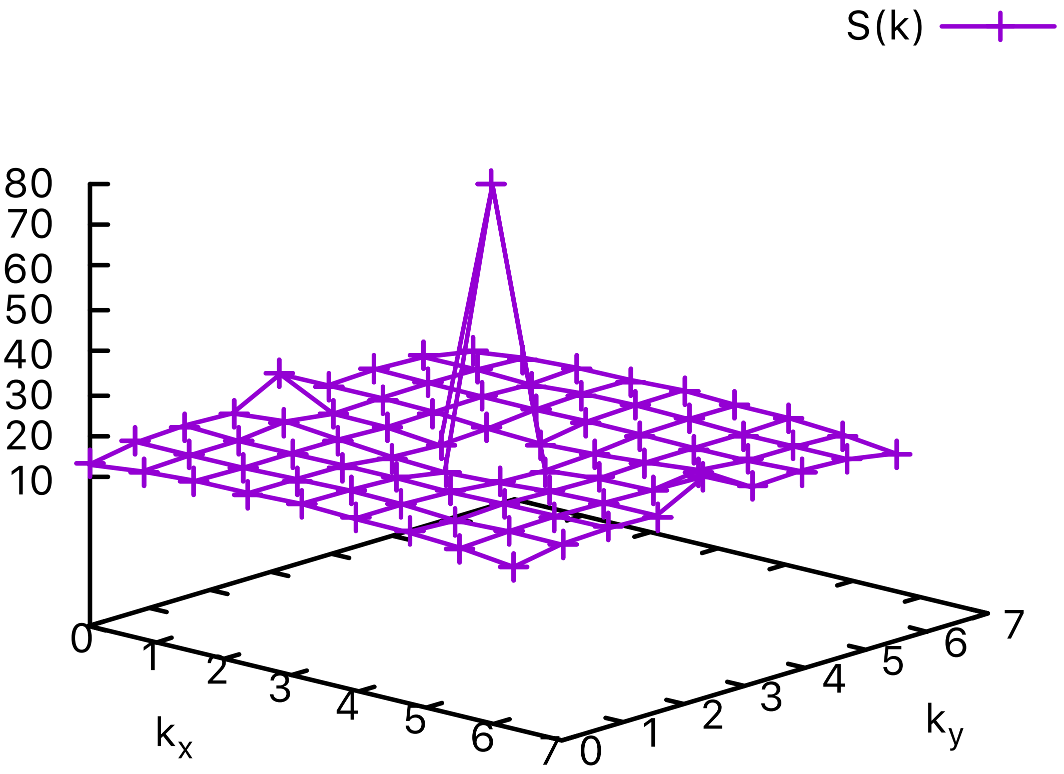


FIG. 1. Structure factor $S_S(\mathbf{k})$, as function of total momentum $k$.

phase diagram, however the overall physical process observed in tVMC is in agreement with the mean-field approach.

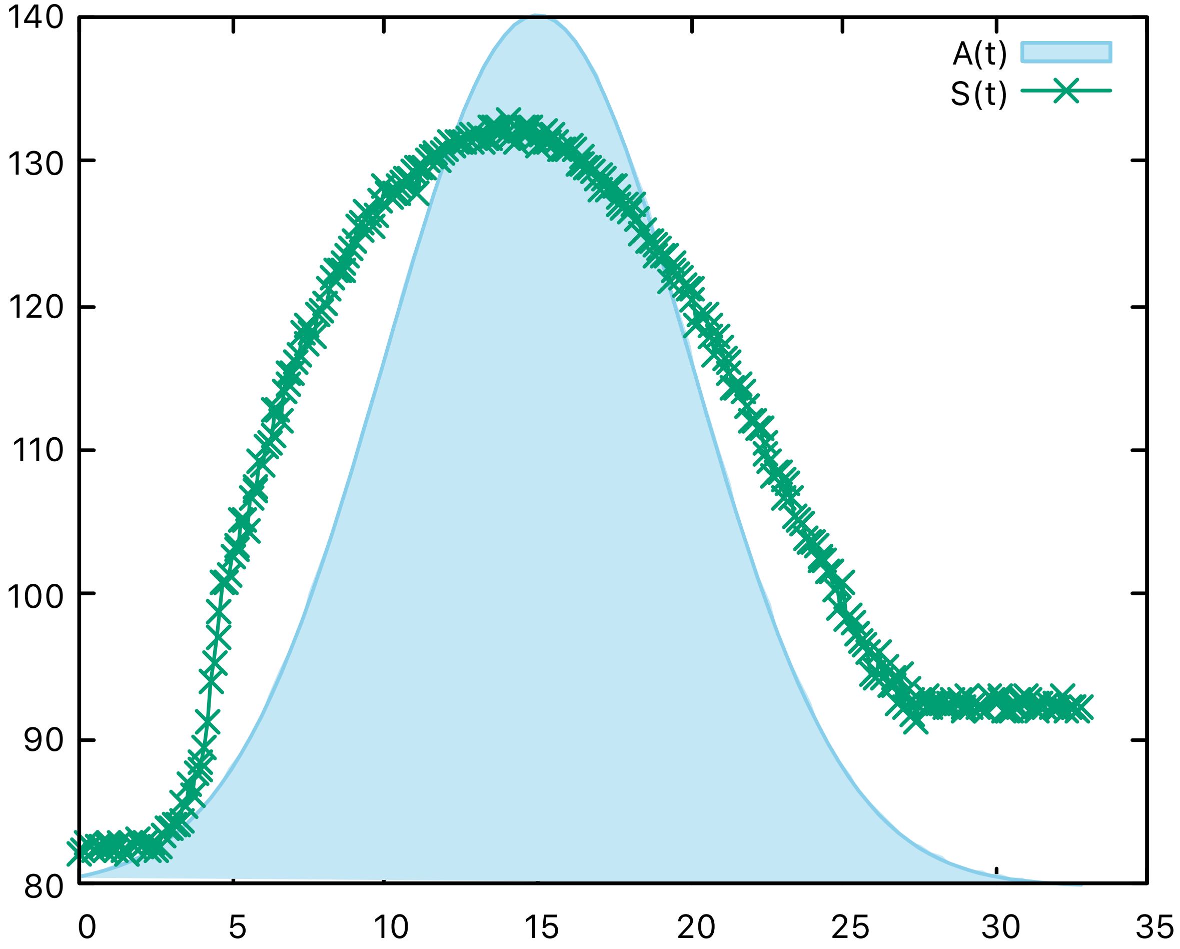


FIG. 2. Time dependence of the peak in the spin structure factor as function of time during the laser pulse. The pulse envelope is shown as a function

[1] Watanabe, H. & Ogata, M. Fermi-surface reconstruction without breakdown of kondo screening at the quantum critical point. *Phys. Rev. Lett.* **99**, 136401 (2007). URL `https://link.aps.org/doi/10.1103/PhysRevLett.99.136401`.
